# Supplementary material for: Medley2K: A Dataset of Medley Transitions
Source: arXiv:2008.11159 source file (2020-08-25)
Supplement: Supplementary file 1 [file appendix.tex]

\section{Appendix}
\subsection{Overview Dataset}
An overview of the topics of the songs can be seen in figure \ref{dataset:wc}.
\begin{figure}[!htb]
\centering
    \includegraphics[width=0.3\textwidth]{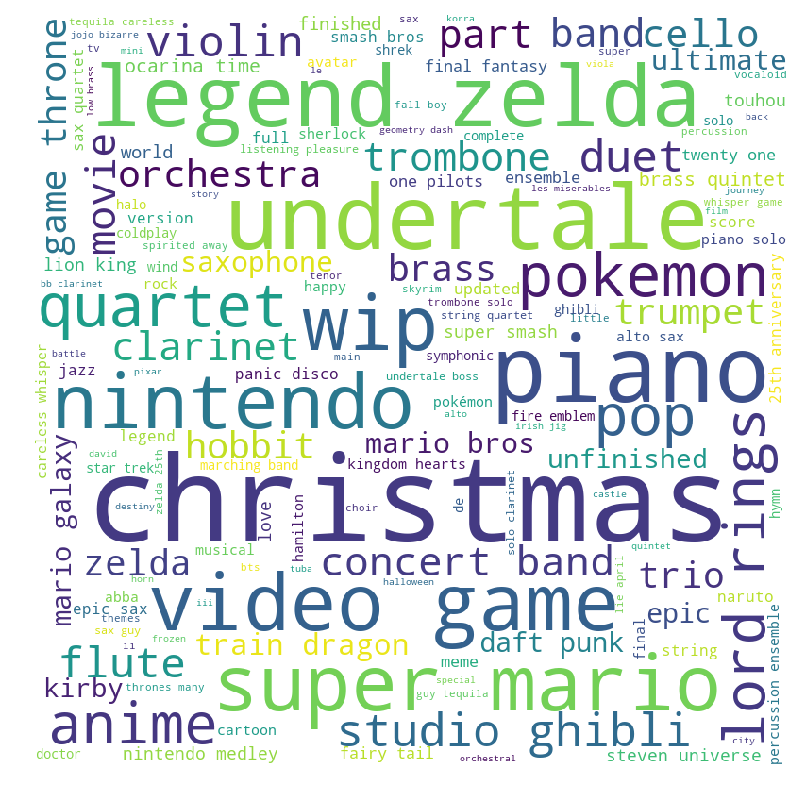}
    \caption{Overview Titles Medley2k}
      \label{dataset:wc}
\end{figure}

\subsection{Filtering}
Maybe we can avoid it, to be thought about in the end
\begin{figure}[!htb]
\centering
    \includegraphics[width=0.3\textwidth]{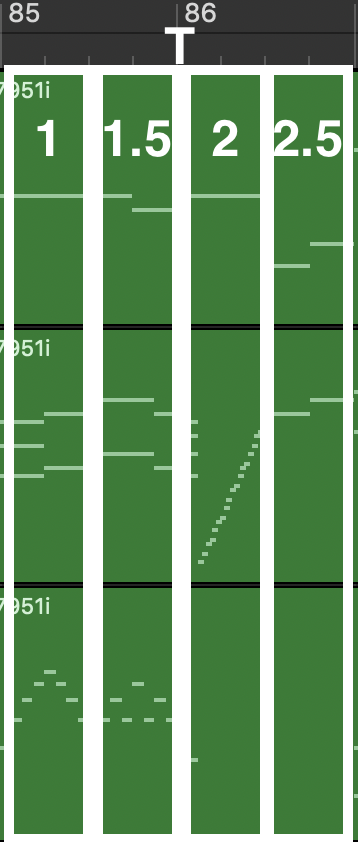}
    \caption{PLACEHOLD IMAGE:Transition filter TODO: nicer image to be found later on...}
      \label{dataset:tf}
\end{figure}

\subsection{Repetition Score}
Music often includes a variety of repetitions that give the song a structure.
To evaluate the amount of repetitions using a simple structure. 
Given a song as $x \in \{0,1....128\}^{b\times q \times p \times v}$ where b is the amount of bars in a song, q is the amount of quarters in a beat e.g. 4 here, p is the amount of pitches and v is the amount of voices.
We now check for each $x[i,:,:,:]$ the amount of times this exact combination occurred.
We define the pattern that occurred the most as $PBar_{max}$.
Additionally we defined for each $x[i,j,:,:]$ the amount of times this exact combination occurred.
We define the pattern that occurred the most as $PQuarter_{max}$.
We now define
\begin{center}
$$
QuarterScore=\frac{PQuarter_{max}}{q*b}
$$
\end{center}
\begin{center}
$$
BarScore=\frac{PBar_{max}}{ b }
$$
\end{center}
Since these scores have a minium which is not 0, e.g. for BarScore the minium is $1/b$ we scale them in to the range $[0,1]$.
The Repetition score can then be defined as
\begin{center}
$RepetitionScore=\frac{QuarterScore+BarScore}{2}$
\end{center}
